# Supplementary material for: Multiparticle Entanglement Resolution Analyzer based on Quantum-Control-Assisted Uncertainty Relation
Source: arXiv:1901.11245 source file (2019-01-31)
Supplement: Supplementary file 1 [file 2019.01.31Supplementary_Material.pdf]

# Supplementary Material for
# Multiparticle Entanglement Resolution Analyzer based on Quantum-Control-Assisted Uncertainty Relation

Shao-Qiang Ma,[1] Xiao Zheng,[1] Guo-Feng Zhang,[1,*] Heng Fan,[2,3,4] Wu-Ming Liu,[2,3,5] and Leong-Chuan Kwek[6,7,8]

[1]*School of Physics, Beihang University, Beijing 100191, China*
[2]*Beijing National Laboratory for Condensed Matter Physics, Institute of Physics, Chinese Academy of Sciences, Beijing 100190, China*
[3]*School of Physical Sciences, University of Chinese Academy of Sciences, Beijing 100190, China*
[4]*CAS Central of Excellence in Topological Quantum Computation, Beijing 100190, China*
[5]*Songshan Lake Materials Laboratory , Dongguan, Guangdong 523808, China*
[6]*Centre for Quantum Technologies, National University of Singapore*
[7]*MajuLab, CNRS-UNS-NUS-NTU International Joint Research Unit, Singapore UMI 3654, Singapore*
[8]*National Institute of Education, Nanyang Technological University, Singapore 637616, Singapore*

(Dated: January 30, 2019)

Assume $O^S$ ($Q^S$) and $|\cdots\rangle^S$ represent the observable $O$ ($Q$) and quantum state of the subsystem $S$, respectively. $O$ and $Q$ stand for two arbitrary observables, and $|\lambda_j\rangle$ ($|\mu_i\rangle$) is an eigenstate of $O$ ($Q$) with $i, j = 1, 2, \cdots, d$ and $d$ being the dimension of the subsystem $S$. $P\left(\rho, O^S := \lambda_j\right)$ [1] is the probability that the measurement result is $\lambda_j$ when we perform the measurement $O$ on the subsystem $S$, and $\rho_{(O^S:=\lambda_j)}$ represents the state after measurement, with $\rho$ being the state of the whole system before the measurement. Here, we should mention that the measurement $O$ means the orthogonal projective measurement in terms of the eigenstates of the operator $O$.

The supplementary material is divided into three sections. The first section is used to prove Eq.(4) in the main text. The second section is devoted to the proof of the multi-quantum-control-assisted uncertainty relation. The related proof of the resolution analyzer for different multiparticle entanglement classes is presented in the third section.

## Section. I. Variance of the measurement result is reduced subject to the given condition

This section is to prove Eq.(4) in the main text:

$$\mathrm{E}\left[\mathrm{V}\left(Q^{S_1}|O^{S_2}\right)\right] \leq \mathrm{V}\left(Q^{S_1}\right).$$

We first introduce a lemma, and then complete the proof based on the lemma.

**Lemma. 1.**

$$\mathrm{E}\left(Q^{S_1}\right) = \mathrm{E}\left[\mathrm{E}\left(Q^{S_1}|O^{S_2}\right)\right],$$

where $\mathrm{E}\left[\mathrm{E}\left(Q^{S_1}|O^{S_2}\right)\right] = \sum_{\lambda_j} P\left(\rho, O^{S_2} := \lambda_j\right)\mathrm{E}\left(Q^{S_1}|O^{S_2} := \lambda_j\right)$ represents the expectation of $\mathrm{E}\left(Q^{S_1}|O^{S_2} := \lambda_j\right)$ in terms of the possibility $P\left(\rho, O^{S_2} := \lambda_j\right)$, with $\mathrm{E}\left(Q^{S_1}|O^{S_2} := \lambda_j\right) = \mathrm{Tr}\left[Q^{S_1}\mathrm{Tr}^{S_2}\left(\rho_{(O^{S_2}:=\lambda_j)}\right)\right]$ being the conditional expectation of $Q^{S_1}$ given that the measurement result of $O^{S_2}$ is $\lambda_j$, and $\mathrm{Tr}^{S_2}\left(\rho_{(O^{S_2}:=\lambda_j)}\right)$ being the partial trace of $\rho_{(O^{S_2}:=\lambda_j)}$ over the basis of the system $S_2$.

*Proof*: Consider a system containing two subsystems $S_1$ and $S_2$, and assume the state of the whole system is $\rho$. We can obtain that [2]:

$$P\left(\rho, O^{S_2} := \lambda_j\right) = \mathrm{Tr}\left[\left(I^{S_1} \otimes |\lambda_j\rangle^{S_2}\langle\lambda_j|^{S_2}\right)\rho\left(I^{S_1} \otimes |\lambda_j\rangle^{S_2}\langle\lambda_j|^{S_2}\right)\right],$$

* gf1978zhang@buaa.edu.cn

where $I^S$ is the identity operator of the system $S$. The state of the whole system after the measurement turns into [2]:

$$\rho_{(O^{S_2}:=\lambda_j)} = \frac{\left(I^{S_1}\otimes|\lambda_j\rangle^{S_2}\langle\lambda_j|^{S_2}\right)\rho\left(I^{S_1}\otimes|\lambda_j\rangle^{S_2}\langle\lambda_j|^{S_2}\right)}{\mathrm{Tr}\left[\left(I^{S_1}\otimes|\lambda_j\rangle^{S_2}\langle\lambda_j|^{S_2}\right)\rho\left(I^{S_1}\otimes|\lambda_j\rangle^{S_2}\langle\lambda_j|^{S_2}\right)\right]}.$$

$$\mathrm{Tr}^{S_2}\left(\rho_{(O^{S_2}:=\lambda_j)}\right) = \frac{\langle\lambda_j|^{S_2}\rho|\lambda_j\rangle^{S_2}}{\mathrm{Tr}\left[\left(I^{S_1}\otimes|\lambda_j\rangle^{S_2}\langle\lambda_j|^{S_2}\right)\rho\left(I^{S_1}\otimes|\lambda_j\rangle^{S_2}\langle\lambda_j|^{S_2}\right)\right]}.$$

Then, one can obtain:

$$\begin{aligned}
\mathrm{E}\left[\mathrm{E}\left(Q^{S_1}|O^{S_2}\right)\right] &= \sum_{\lambda_j} P\left(\rho, O^{S_2}:=\lambda_j\right)\mathrm{E}\left(Q^{S_1}|O^{S_2}:=\lambda_j\right)\\
&= \sum_{\lambda_j}\mathrm{Tr}\left[\left(I^{S_1}\otimes|\lambda_j\rangle^{S_2}\langle\lambda_j|^{S_2}\right)\rho\left(I^{S_1}\otimes|\lambda_j\rangle^{S_2}\langle\lambda_j|^{S_2}\right)\right]\mathrm{Tr}\left[Q^{S_1}\,\mathrm{Tr}^{S_2}\left(\rho_{(O^{S_2}:=\lambda_j)}\right)\right]\\
&= \sum_{\mu_i}\langle\mu_i|^{S_1}Q^{S_1}\left(\sum_{\lambda_j}\langle\lambda_j|^{S_2}\rho|\lambda_j\rangle^{S_2}\right)|\mu_i\rangle^{S_1}\\
&= \mathrm{Tr}\left[Q^{S_1}\,\mathrm{Tr}^{S_2}(\rho)\right] = \mathrm{E}\left(Q^{S_1}\right).
\end{aligned}$$

Thus the proof of Lemma. 1 is completed.

Based on Lemma.1, we have:

$$\begin{aligned}
\mathrm{V}\left(Q^{S_1}\right) - \mathrm{E}\left[\mathrm{V}\left(Q^{S_1}|O^{S_2}\right)\right] &= \mathrm{E}\left({Q^{S_1}}^2\right) - \left[\mathrm{E}\left(Q^{S_1}\right)\right]^2 - \mathrm{E}\left[\mathrm{V}\left(Q^{S_1}|O^{S_2}\right)\right]\\
&= \mathrm{E}\left[\mathrm{E}\left({Q^{S_1}}^2|O^{S_2}\right)\right] - \left\{\mathrm{E}\left[\mathrm{E}\left(Q^{S_1}|O^{S_2}\right)\right]\right\}^2 - \mathrm{E}\left[\mathrm{V}\left(Q^{S_1}|O^{S_2}\right)\right]\\
&= \sum_{\lambda_j} P\left(\rho, O^{S_2}:=\lambda_j\right)\left[\mathrm{E}\left(Q^{S_1}|O^{S_2}:=\lambda_j\right)\right]^2 - \left\{\mathrm{E}\left[\mathrm{E}\left(Q^{S_1}|O^{S_2}\right)\right]\right\}^2\\
&= \mathrm{V}\left[\mathrm{E}\left(Q^{S_1}|O^{S_2}\right)\right]\\
&\geq 0,
\end{aligned}$$

where $\mathrm{V}\left[\mathrm{E}\left(Q^{S_1}|O^{S_2}\right)\right] = \sum_{\lambda_j} P\left(\rho, O^{S_2}:=\lambda_j\right)\left\{\mathrm{E}\left(Q^{S_1}|O^{S_2}:=\lambda_j\right) - \mathrm{E}\left[\mathrm{E}\left(Q^{S_1}|O^{S_2}\right)\right]\right\}^2$ is the variance of $\mathrm{E}\left(Q^{S_1}|O^{S_2}:=\lambda_j\right)$ in terms of the possibility $P\left(\rho, O^{S_2}:=\lambda_j\right)$. Thus, we obtain Eq.(4) in the main text.

**Section. II. Multi-Quantum-Control-Assisted Uncertainty Relation**

This Section is mainly used to prove the multi-quantum-control-assisted uncertainty relation, which reads:

$$\sum_{k=1}^{K}\mathrm{E}\left[\mathrm{V}\left(Q_k^A|O_k^{C_1},\cdots,O_k^{C_N}\right)\right] \geq L_{tra} - \sum_{k=1}^{K}\mathrm{V}\left[\mathrm{E}\left(Q_k^A|O_k^{C_1}\right)\right] - \sum_{k=1}^{K}\sum_{n=2}^{N}\mathrm{E}\left[\mathrm{V}\left(\mathrm{E}\left[Q_k^A|O_k^{C_n}\right]|O_k^{C_1},\cdots,O_k^{C_{n-1}}\right)\right].$$

In the following, we first introduce two lemmas and a theorem.

**Lemma. 2.**

$$\mathrm{E}\left(Q^A|O^{C_1}:=\lambda_j\right) = \mathrm{E}\left[\mathrm{E}\left(Q^A|O^{C_2}\right)|O^{C_1}:=\lambda_j\right],$$

where $\mathrm{E}\left[\mathrm{E}\left(Q^A|O^{C_2}\right)|Q^{C_1}:=\lambda_j\right]$ is the conditional expectation of $\mathrm{E}\left(Q^A|O^{C_2}:=\lambda_m\right)$ in terms of the possibility $P\left(\rho_{(O^{C_1}:=\lambda_j)}, O^{C_2}:=\lambda_m\right)$ on the condition that the measurement $O^{C_1}$ has been performed and the corresponding result is obtained as $\lambda_j$. Thus, $\mathrm{E}\left[\mathrm{E}\left(Q^A|O^{C_2}\right)|O^{C_1}:=\lambda_j\right] = \sum_{\lambda_m} P\left(\rho_{(O^{C_1}:=\lambda_j)}, O^{C_2}:=\lambda_m\right)\mathrm{E}\left(Q^A|O^{C_2}:=\lambda_m\right)$, where $\mathrm{E}\left(Q^A|O^{C_2}:=\lambda_m\right)$ is calculated on the state

$\rho_{(O^{C_1}:=\lambda_j)}$, with the $\rho$ being the state of the whole system before measurement.

*Proof*: Considering a system which contains three subsystems $A, C_1$ and $C_2$ , we have:

$$\rho_{(O^{C_1}:=\lambda_j)} = \tilde{\rho} = \frac{\left(I^A \otimes |\lambda_j\rangle^{C_1}\langle\lambda_j|^{C_1} \otimes I^{C_2}\right)\rho\left(I^A \otimes |\lambda_j\rangle^{C_1}\langle\lambda_j|^{C_1} \otimes I^{C_2}\right)}{\mathrm{Tr}\left[\left(I^A \otimes |\lambda_j\rangle^{C_1}\langle\lambda_j|^{C_1} \otimes I^{C_2}\right)\rho\left(I^A \otimes |\lambda_j\rangle^{C_1}\langle\lambda_j|^{C_1} \otimes I^{C_2}\right)\right]}.$$

We perform the measurement $O^{C_2}$ on the state $\rho_{(O^{C_1}:=\lambda_j)}$, and the probability, that the measurement results is $\lambda_m$, is obtained:

$$\begin{aligned}P\left(\rho_{(O^{C_1}:=\lambda_j)}, O^{C_2} := \lambda_m\right) &= \mathrm{Tr}\left[\left(I^A \otimes I^{C_1} \otimes |\lambda_m\rangle^{C_2}\langle\lambda_m|^{C_2}\right)\tilde{\rho}\left(I^A \otimes I^{C_1} \otimes |\lambda_m\rangle^{C_2}\langle\lambda_m|^{C_2}\right)\right]\\ &= \frac{\mathrm{Tr}\left[\left(I^A \otimes |\lambda_j\rangle^{C_1}\langle\lambda_j|^{C_1} \otimes |\lambda_m\rangle^{C_2}\langle\lambda_m|^{C_2}\right)\rho\left(I^A \otimes |\lambda_j\rangle^{C_1}\langle\lambda_j|^{C_1} \otimes |\lambda_m\rangle^{C_2}\langle\lambda_m|^{C_2}\right)\right]}{\mathrm{Tr}\left[\left(I^A \otimes |\lambda_j\rangle^{C_1}\langle\lambda_j|^{C_1} \otimes I^{C_2}\right)\rho\left(I^A \otimes |\lambda_j\rangle^{C_1}\langle\lambda_j|^{C_1} \otimes I^{C_2}\right)\right]}.\end{aligned}$$

The state after the measurements becomes:

$$\tilde{\rho}_{(O^{C_2}:=\lambda_m)} = \frac{\left(I^A \otimes I^{C_1} \otimes |\lambda_m\rangle^{C_2}\langle\lambda_m|^{C_2}\right)\tilde{\rho}\left(I^A \otimes I^{C_1} \otimes |\lambda_m\rangle^{C_2}\langle\lambda_m|^{C_2}\right)}{\mathrm{Tr}\left[(I^A \otimes I^{C_1} \otimes |\lambda_m\rangle^{C_2}\langle\lambda_m|^{C_2})\,\tilde{\rho}\,(I^A \otimes I^{C_1} \otimes |\lambda_m\rangle^{C_2}\langle\lambda_m|^{C_2})\right]}.$$

Then we have:

$$\begin{aligned}\mathrm{E}\left[\mathrm{E}\left(Q^A|O^{C_2}\right)|O^{C_1} := \lambda_j\right] &= \sum_{\lambda_m} P\left(\rho_{(O^{C_1}:=\lambda_j)}, O^{C_2} := \lambda_m\right)\mathrm{E}\left(Q^A|O^{C_2} := \lambda_m\right)\\ &= \sum_{\lambda_m} P\left(\rho_{(O^{C_1}:=\lambda_j)}, O^{C_2} := \lambda_m\right)\mathrm{Tr}\left[Q^A \mathrm{Tr}^{C_1,C_2}\left(\tilde{\rho}_{(O^{C_2}:=\lambda_m)}\right)\right]\\ &= \sum_{\lambda_m} \mathrm{Tr}\left[Q^A \frac{\langle\lambda_j|^{C_1}\langle\lambda_m|^{C_2}\rho|\lambda_j\rangle^{C_1}|\lambda_m\rangle^{C_2}}{\mathrm{Tr}\left[\left(I^A \otimes |\lambda_j\rangle^{C_1}\langle\lambda_j|^{C_1} \otimes I^{C_2}\right)\rho\left(I^A \otimes |\lambda_j\rangle^{C_1}\langle\lambda_j|^{C_1} \otimes I^{C_2}\right)\right]}\right]\\ &= \mathrm{Tr}\left[Q^A\, \mathrm{Tr}^{C_1,C_2}\left(\rho_{(O^{C_1}:=\lambda_j)}\right)\right]\\ &= \mathrm{E}\left(Q^A|O^{C_1} := \lambda_j\right).\end{aligned}$$

Thus the Lemma. 2 is obtained.

**Lemma. 3.**

$$\mathrm{E}\left(\mathrm{E}\left[\mathrm{V}\left(Q^A|O^{C_2}\right)|O^{C_1}\right]\right) = \mathrm{E}\left[\mathrm{V}\left(Q^A|O^{C_1}, O^{C_2}\right)\right].$$

where $\mathrm{E}\left(\mathrm{E}\left[\mathrm{V}\left(Q^A|O^{C_2}\right)|O^{C_1}\right]\right) = \sum_{\lambda_j} P\left(\rho, O^{C_1} := \lambda_j\right)\mathrm{E}\left[\mathrm{V}\left(Q^A|O^{C_2}\right)|O^{C_1} := \lambda_j\right]$ is the expectation of $\mathrm{E}\left[\mathrm{V}\left(Q^A|O^{C_2}\right)|O^{C_1} := \lambda_j\right]$ in terms of the possibility $P\left(\rho, O^{C_1} := \lambda_j\right)$. $\mathrm{E}\left[\mathrm{V}\left(Q^A|O^{C_2}\right)|O^{C_1} := \lambda_j\right] = \sum_{\lambda_m} P\left(\rho_{O^{C_1}:=\lambda_j}, O^{C_2} := \lambda_m\right)\mathrm{V}\left(Q^A|O^{C_2} := \lambda_m\right)$, where $\mathrm{V}\left(Q^A|O^{C_2} := \lambda_m\right)$ are calculated on the state $\rho_{(O^{C_1}:=\lambda_j)}$.

*Proof:* Similar to the proof of Lemma. 2, we consider a system containing three subsystems $A$, $C_1$ and $C_2$. Then, we obtain:

$$\begin{aligned}P\left(\rho_{(O^{C_1}:=\lambda_j)}, O^{C_2} := \lambda_m\right) &= \mathrm{Tr}\left[\left(I^A \otimes I^{C_1} \otimes |\lambda_m\rangle^{C_2}\langle\lambda_m|^{C_2}\right)\tilde{\rho}\left(I_A \otimes I^{C_1} \otimes |\lambda_m\rangle^{C_2}\langle\lambda_m|^{C_2}\right)\right]\\ &= \frac{\mathrm{Tr}\left[\left(I^A \otimes |\lambda_j\rangle^{C_1}\langle\lambda_j|^{C_1} \otimes |\lambda_m\rangle^{C_2}\langle\lambda_m|^{C_2}\right)\rho\left(I^A \otimes |\lambda_j\rangle^{C_1}\langle\lambda_j|^{C_1} \otimes |\lambda_m\rangle^{C_2}\langle\lambda_m|^{C_2}\right)\right]}{\mathrm{Tr}\left[\left(I^A \otimes |\lambda_j\rangle^{C_1}\langle\lambda_j|^{C_1} \otimes I^{C_2}\right)\rho\left(I^A \otimes |\lambda_j\rangle^{C_1}\langle\lambda_j|^{C_1} \otimes I^{C_2}\right)\right]}.\end{aligned}$$

$$\rho_{(O^{C_1}:=\lambda_j)} = \tilde{\rho} = \frac{\left(I^A \otimes |\lambda_j\rangle^{C_1}\langle\lambda_j|^{C_1} \otimes I^{C_2}\right)\rho\left(I^A \otimes |\lambda_j\rangle^{C_1}\langle\lambda_j|^{C_1} \otimes I^{C_2}\right)}{\mathrm{Tr}\left[\left(I^A \otimes |\lambda_j\rangle^{C_1}\langle\lambda_j|^{C_1} \otimes I^{C_2}\right)\rho\left(I^A \otimes |\lambda_j\rangle^{C_1}\langle\lambda_j|^{C_1} \otimes I^{C_2}\right)\right]},$$

$$P\left(\rho_{(O^{C_1}:=\lambda_j)}, O^{C_2} := \lambda_m\right) = \mathrm{Tr}\left[\left(I^A \otimes I^{C_1} \otimes |\lambda_m\rangle^{C_2}\langle\lambda_m|^{C_2}\right)\tilde{\rho}\left(I^A \otimes I^{C_1} \otimes |\lambda_m\rangle^{C_2}\langle\lambda_m|^{C_2}\right)\right],$$

where $P\left(\rho_{(O^{C_1}:=\lambda_j)}, O^{C_2} := \lambda_m\right)$ represents the probability that the measurement result is $\lambda_m$ when we perform the measurement $O^{C_2}$ on the state $\rho_{(O^{C_1}:=\lambda_j)}$. The state after the measurements becomes:

$$\tilde{\rho}_{(O^{C_2}:=\lambda_m)} = \frac{\left(I^A \otimes I^{C_1} \otimes |\lambda_m\rangle^{C_2}\langle\lambda_m|^{C_2}\right)\tilde{\rho}\left(I^A \otimes I^{C_1} \otimes |\lambda_m\rangle^{C_2}\langle\lambda_m|^{C_2}\right)}{\mathrm{Tr}\left[\left(I^A \otimes I^{C_1} \otimes |\lambda_m\rangle^{C_2}\langle\lambda_m|^{C_2}\right)\tilde{\rho}\left(I^A \otimes I^{C_1} \otimes |\lambda_m\rangle^{C_2}\langle\lambda_m|^{C_2}\right)\right]}.$$

Meanwhile,we have:

$$\begin{aligned}
\mathrm{Tr}^{C_1,C_2}\left(\tilde{\rho}_{(O^{C_2}:=\lambda_m)}\right) &= \frac{\sum_{\lambda_l}\langle\lambda_l|^{C_1}\langle\lambda_m|^{C_2}\tilde{\rho}|\lambda_l\rangle^{C_1}|\lambda_m\rangle^{C_2}}{\mathrm{Tr}\left[\left(I^A \otimes I^{C_1} \otimes |\lambda_m\rangle^{C_2}\langle\lambda_m|^{C_2}\right)\tilde{\rho}\left(I^A \otimes I^{C_1} \otimes |\lambda_m\rangle^{C_2}\langle\lambda_m|^{C_2}\right)\right]} \\
&= \frac{\langle\lambda_j|^{C_1}\langle\lambda_m|^{C_2}\rho|\lambda_j\rangle^{C_1}|\lambda_m\rangle^{C_2}}{\mathrm{Tr}\left[\left(I^A \otimes |\lambda_j\rangle^{C_1}\langle\lambda_j|^{C_1} \otimes |\lambda_m\rangle^{C_2}\langle\lambda_m|^{C_2}\right)\rho\left(I^A \otimes |\lambda_j\rangle^{C_1}\langle\lambda_j|^{C_1} \otimes |\lambda_m\rangle^{C_2}\langle\lambda_m|^{C_2}\right)\right]} \\
&= \mathrm{Tr}^{C_1,C_2}\left(\rho_{(O^{C_1}:=\lambda_j, O^{C_2}:=\lambda_m)}\right),
\end{aligned}$$

where

$$\rho_{(O^{C_1}:=\lambda_j, O^{C_2}:=\lambda_m)} = \frac{\left(I^A \otimes |\lambda_j\rangle^{C_1}\langle\lambda_j|^{C_1} \otimes |\lambda_m\rangle^{C_2}\langle\lambda_m|^{C_2}\right)\rho\left(I^A \otimes |\lambda_j\rangle^{C_1}\langle\lambda_j|^{C_1} \otimes |\lambda_m\rangle^{C_2}\langle\lambda_m|^{C_2}\right)}{\mathrm{Tr}\left[\left(I^A \otimes |\lambda_j\rangle^{C_1}\langle\lambda_j|^{C_1} \otimes |\lambda_m\rangle^{C_2}\langle\lambda_m|^{C_2}\right)\rho\left(I^A \otimes |\lambda_j\rangle^{C_1}\langle\lambda_j|^{C_1} \otimes |\lambda_m\rangle^{C_2}\langle\lambda_m|^{C_2}\right)\right]}.$$

Combining the formulas above, one can obtain:

$$\begin{aligned}
&\mathrm{E}\left(\mathrm{E}\left[\mathrm{V}\left(Q^A|O^{C_2}\right)|O^{C_1}\right]\right) \\
&= \sum_{\lambda_j} P\left(\rho, O^{C_1} := \lambda_j\right)\mathrm{E}\left[\mathrm{V}\left(Q^A|O^{C_2}\right)|O^{C_1} := \lambda_j\right] \\
&= \sum_{\lambda_j} P\left(\rho, O^{C_1} := \lambda_j\right)\sum_{\lambda_m} P\left(\tilde{\rho}, O^{C_2} := \lambda_m\right)\mathrm{Var}\left(Q^A, \mathrm{Tr}^{C_1C_2}\left(\tilde{\rho}_{(O^{C_2}:=\lambda_m)}\right)\right) \\
&= \sum_{\lambda_j}\sum_{\lambda_m}\mathrm{Tr}\left[\left(I^A \otimes |\lambda_j\rangle^{C_1}\langle\lambda_j|^{C_1} \otimes |\lambda_m\rangle^{C_2}\langle\lambda_m|^{C_2}\right)\rho\left(I^A \otimes |\lambda_j\rangle^{C_1}\langle\lambda_j|^{C_1} \otimes |\lambda_m\rangle^{C_2}\langle\lambda_m|^{C_2}\right)\right]\mathrm{Var}\left(Q^A, \mathrm{Tr}^{C_1C_2}\left(\tilde{\rho}_{(O^{C_2}:=\lambda_m)}\right)\right) \\
&= \sum_{\lambda_j}\sum_{\lambda_m}\mathrm{Tr}\left[\left(I^A \otimes |\lambda_j\rangle^{C_1}\langle\lambda_j|^{C_1} \otimes |\lambda_m\rangle^{C_2}\langle\lambda_m|^{C_2}\right)\rho\left(I^A \otimes |\lambda_j\rangle^{C_1}\langle\lambda_j|^{C_1} \otimes |\lambda_m\rangle^{C_2}\langle\lambda_m|^{C_2}\right)\right]\mathrm{Var}\left(Q^A, \mathrm{Tr}^{C_1,C_2}\left(\rho_{(O^{C_1}:=\lambda_j, O^{C_2}:=\lambda_m)}\right)\right) \\
&= \sum_{\lambda_j}\sum_{\lambda_m} P\left(\rho, O^{C_1} := \lambda_j, O^{C_2} := \lambda_m\right)\mathrm{Var}\left(Q^A, \mathrm{Tr}^{C_1,C_2}\left(\rho_{(O^{C_1}:=\lambda_j, O^{C_2}:=\lambda_m)}\right)\right) \\
&= \mathrm{E}\left[\mathrm{V}\left(Q^A|O^{C_1}, O^{C_2}\right)\right].
\end{aligned}$$

Thus, we obtain Lemma. 3.

**Theorem. 1:** The sum form variance-based uncertainty relation for $K$ incompatible observables is [3]:

$$\sum_{k=1}^{K}\mathrm{V}\left(Q_k^A\right) \geq L_{tra},$$

where $L_{tra}$ represents a state-dependent lower bound. According to Ref. [3], by introducing a pair of generalized-incompatible operators, the lower bound $L_{tra}$ can be guaranteed non-trivial when there exists no common eigenstate between $Q_1^A, Q_2^A, \cdots, Q_K^A$. Moreover, the lower bound $L_{tra}$ can be exactly equal to $\sum_{k=1}^{K}\mathrm{V}(Q_k^A)$ when a specific number of auxiliary operators are introduced.

**The proof of multi-quantum-control-assisted uncertainty relation:** Based on Lemma.1, we have:

$$\begin{aligned} \mathrm{V}\left(Q^A\right) &= \mathrm{E}\left({Q^A}^2\right) - \left[\mathrm{E}\left(Q^A\right)\right]^2 \\ &= \mathrm{E}\left[\mathrm{E}\left({Q^A}^2|O^{C_1}\right)\right] - \left\{\mathrm{E}\left[\mathrm{E}\left(Q^A|O^{C_1}\right)\right]\right\}^2 \\ &= \mathrm{E}\left[\mathrm{V}\left(Q^A|O^{C_1}\right)\right] + \mathrm{E}\left[\mathrm{E}\left(Q^A|O^{C_1}\right)^2\right] - \left\{\mathrm{E}\left[\mathrm{E}\left(Q^A|O^{C_1}\right)\right]\right\}^2 \\ &= \mathrm{E}\left[\mathrm{V}\left(Q^A|O^{C_1}\right)\right] + \mathrm{V}\left[\mathrm{E}\left(Q^A|O^{C_1}\right)\right]. \end{aligned} \tag{S1}$$

Then, combining (S1) and theorem.1, one can obtain the uncertainty relation based on one control system:

$$\sum_{k=1}^{K} \mathrm{E}\left[\mathrm{V}\left(Q_k^A|O_k^{C_1}, \cdots, O_k^{C_N}\right)\right] \geq L_{tra} - \sum_{k=1}^{K} \mathrm{V}\left[\mathrm{E}\left(Q_k^A|O_k^{C_1}\right)\right].$$

Similarly, according to Lemma.2, one can obtain:

$$\begin{aligned} \mathrm{V}\left(Q^A|O^{C_1} := \lambda_j\right) &= \mathrm{E}\left({Q^A}^2|O^{C_1} := \lambda_j\right) - \left\{\mathrm{E}\left(Q^A|O^{C_1} := \lambda_j\right)\right\}^2 \\ &= \mathrm{E}\left[\mathrm{E}\left({Q^A}^2|O^{C_2}\right)|O^{C_1} := \lambda_j\right] - \left\{\mathrm{E}\left[\mathrm{E}\left(Q^A|O^{C_2}\right)|O^{C_1} := \lambda_j\right]\right\}^2 \\ &= \mathrm{E}\left[\mathrm{V}\left(Q^A|O^{C_2}\right)|O^{C_1} := \lambda_j\right] + \mathrm{E}\left[\mathrm{E}\left(Q^A|O^{C_2}\right)^2|O^{C_1} := \lambda_j\right] - \left\{\mathrm{E}\left[\mathrm{E}\left(Q^A|O^{C_2}\right)|O^{C_1} := \lambda_j\right]\right\}^2 \\ &= \mathrm{E}\left[\mathrm{V}\left(Q^A|O^{C_2}\right)|O^{C_1} := \lambda_j\right] + \mathrm{V}\left[\mathrm{E}\left(Q^A|O^{C_2}\right)|O^{C_1} := \lambda_j\right]. \end{aligned} \tag{S2}$$

Substituting (S2) into (S1) and taking advantage of Lemma.3, we obtain:

$$\mathrm{V}\left(Q^A\right) = \mathrm{E}\left[\mathrm{V}\left(Q^A|O^{C_1}, O^{C_2}\right)\right] + \mathrm{E}\left(\mathrm{V}\left[\mathrm{E}\left(Q^A|O^{C_2}\right)|O^{C_1}\right]\right) + \mathrm{V}\left[\mathrm{E}\left(Q^A|O^{C_1}\right)\right]. \tag{S3}$$

where $\mathrm{E}\left(\mathrm{V}\left[\mathrm{E}\left(Q^A|O^{C_2}\right)|O^{C_1}\right]\right) = \sum_{\lambda_j} P\left(\rho, O^{C_1} := \lambda_j\right)\mathrm{V}\left[\mathrm{E}\left(Q^A|O^{C_2}\right)|O^{C_1} := \lambda_j\right]$ is the expectation of $\mathrm{V}\left[\mathrm{E}\left(Q^A|O^{C_2}\right)|O^{C_1} := \lambda_j\right]$ in terms of the possibility $P\left(\rho, O^{C_1} := \lambda_j\right)$, with

$$\mathrm{V}\left[\mathrm{E}\left(Q^A|O^{C_2}\right)|O^{C_1} := \lambda_j\right] = \sum_{\lambda_m} P\left(\rho_{(O^{C_1}:=\lambda_j)}, O^{C_2} := \lambda_m\right)\left[\mathrm{E}\left(Q^A|O^{C_2} := \lambda_m\right) - \sum_{\lambda_{m'}} P\left(\rho_{(O^{C_1}:=\lambda_j)}, O^{C_2} := \lambda_{m'}\right)\mathrm{E}\left(Q^A|O^{C_2} := \lambda_{m'}\right)\right]^2,$$

and $\mathrm{E}\left(Q^A|O^{C_2} := \lambda_m\right)$ being calculated on the state $\rho_{(O^{C_1}:=\lambda_j)}$. Based on Eq.(S3) and theorem.1, we can obtain the uncertainty relation based on two control systems:

$$\sum_{k=1}^{K} \mathrm{E}\left[\mathrm{V}\left(Q_k^A|O_k^{C_1}, \cdots, O_k^{C_N}\right)\right] \geq L_{tra} - \sum_{k=1}^{K} \mathrm{V}\left[\mathrm{E}\left(Q_k^A|O_k^{C_1}\right)\right] - \sum_{k=1}^{K} \mathrm{E}\left[\mathrm{V}\left(\mathrm{E}\left[Q_k^A|O_k^{C_2}\right]|O_k^{C_1}\right)\right].$$

Similarly, we can obtain:

$$\mathrm{V}\left(Q^A\right) = \mathrm{E}\left[\mathrm{V}\left(Q^A|O^{C_1}, O^{C_2}, \ldots, O^{C_N}\right)\right] + \sum_{n=2}^{N} \mathrm{E}\left[\mathrm{V}\left(\mathrm{E}\left[Q_k^A|O_k^{C_n}\right]|O_k^{C_1}, O_k^{C_2}, \ldots, O_k^{C_{n-1}}\right)\right] + \mathrm{V}\left[\mathrm{E}\left(Q^A|O^{C_1}\right)\right]. \tag{S4}$$

After proper deformation, (S4) becomes:

$$\mathrm{E}\left[\mathrm{V}\left(Q^A|O^{C_1}, O^{C_2}, \ldots, O^{C_N}\right)\right] = \mathrm{V}\left(Q^A\right) - \sum_{n=2}^{N} \mathrm{E}\left[\mathrm{V}\left(\mathrm{E}\left[Q_k^A|O_k^{C_n}\right]|O_k^{C_1}, O_k^{C_2}, \ldots, O_k^{C_{n-1}}\right)\right] - \mathrm{V}\left[\mathrm{E}\left(Q^A|O^{C_1}\right)\right]. \tag{S5}$$

Based on (S5) and Theorem.1, we can obtain the multi-quantum-control-assisted uncertainty relation:

$$\sum_{k=1}^{K} \mathrm{E}\left[\mathrm{V}\left(Q_k^A|O_k^{C_1},\cdots,O_k^{C_N}\right)\right] \geq L_{tra} - \sum_{k=1}^{K} \mathrm{V}\left[\mathrm{E}\left(Q_k^A|O_k^{C_1}\right)\right] - \sum_{k=1}^{K}\sum_{n=2}^{N} \mathrm{E}\left[\mathrm{V}\left(\mathrm{E}\left[Q_k^A|O_k^{C_n}\right]|O_k^{C_1},\cdots,O_k^{C_{n-1}}\right)\right].$$

where

$$\mathrm{E}\left[\mathrm{V}\left(\mathrm{E}\left[Q_k^A|O_k^{C_n}\right]|O_k^{C_1},\cdots,O_k^{C_{n-1}}\right)\right] = \sum_{\lambda_j} P\left(\rho, O_k^{C_1} := \lambda_j^{(k)},\cdots,O_k^{C_{n-1}} := \lambda_l^{(k)}\right)\mathrm{V}\left(\mathrm{E}\left[Q_k^A|O_k^{C_n}\right]|O_k^{C_1} := \lambda_j^{(k)},\cdots,O_k^{C_{n-1}} := \lambda_l^{(k)}\right),$$

and

$$\begin{aligned}&\mathrm{V}\left(\mathrm{E}\left[Q_k^A|O_k^{C_n}\right]|O_k^{C_1} := \lambda_j^{(k)},\cdots,O_k^{C_{n-1}} := \lambda_l^{(k)}\right)\\ &= \sum_{\lambda_m^{(k)}} P\left(\rho_{\left(O_k^{C_1}:=\lambda_j^{(k)},\cdots,O_k^{C_{n-1}}:=\lambda_l^{(k)}\right)}, O_k^{C_n} := \lambda_m^{(k)}\right)\left[\mathrm{E}\left(Q^A|O_k^{C_n} := \lambda_m^{(k)}\right) - \sum_{\lambda_{m'}^{k}} P\left(\rho_{\left(O_k^{C_1}:=\lambda_j^{(k)},\cdots,O_k^{C_{n-1}}:=\lambda_l^{(k)}\right)}, O_k^{C_n} := \lambda_{m'}^{(k)}\right)\mathrm{E}\left(Q^A|O_k^{C_n} := \lambda_{m'}^{(k)}\right)\right]^2,\end{aligned}$$

with $\mathrm{E}\left(Q^A|O_k^{C_n} := \lambda_m^{(k)}\right)$ being calculated on the state $\rho_{\left(O_k^{C_1}:=\lambda_j^{(k)},\cdots,O_k^{C_{n-1}}:=\lambda_l^{(k)}\right)}$. Remarkably, the new uncertainty relation will be become equality when $\sum_{k=1}^{K}\mathrm{V}(Q_k^A) = L_{tra}$. That is to say, the multi-quantum-control-assisted uncertainty relation will be become equality when a specific number of auxiliary operators are introduced. Then the proof of the new uncertainty relation is completed.

## Section. III. Resolution Analyzer for Multiparticle Entanglement Classes

Here we will use the reduction to absurdity to prove that the pure state of $N+1$ particles is a genuinely multiparticle entangled state when $\mathcal{L}_0 > \mathcal{L}_1 > \cdots > \mathcal{L}_N$.

*Proof:* Assume that (i) the state of the system is not genuinely multiparticle entangled, which means the state of interest is 2-separable, and (ii)$\mathcal{L}_0 > \mathcal{L}_1 > \cdots > \mathcal{L}_N$. Then, we deduce that there exists a control system, for instance $C_n$, the state of which is separable with the measured system. That means[4, 5]:

$$\mathrm{E}\left(Q_k^A|O_k^{C_n} := \lambda_j^{(k)}\right) = \mathrm{E}\left(Q_k^A\right), \tag{S7}$$

with $\lambda_j^{(k)}$ being an eigenstate of $O_k$. Then, one can obtain:

$$\mathcal{L}_{n-1} - \mathcal{L}_n = \sum_{k=1}^{K} \mathrm{E}\left[\mathrm{V}\left(\mathrm{E}\left[Q_k^A|O_k^{C_n}\right]|O_k^{C_1},O_k^{C_2},\ldots,O_k^{C_{N-1}}\right)\right] \equiv 0, \tag{S8}$$

for $n \geq 2$, and [4, 5]:

$$\mathcal{L}_0 - \mathcal{L}_1 = \sum_{k=1}^{K} \mathrm{V}\left[\mathrm{E}\left(Q_k^A|O_k^{C_1}\right)\right] \equiv 0, \tag{S9}$$

for $n = 1$. Obviously, this conclusion and assumption (ii) are contradictory with each other, and thus we obtain that the state of $N+1$ particles is a genuinely multiparticle entangled state when $\mathcal{L}_0 > \mathcal{L}_1 > \cdots > \mathcal{L}_N$.

Similarly, one can deduce that there exist at least $m$ particles which are entangled with each other when the number of split MERLs is equal to $m$. That is to say, the pure state can be $(N+2-m)$-separable, $(N+1-m)$-separable, $\cdots$, 2-separable or genuinely multiparticle entangled when $m$ split MERLs have been detected.

[1] In the main text, we use the $P\left(O^S := \lambda_j\right)$ to denote the possibility that the measurement result is $\lambda_j$ when we perform the measurement $O$ on the subsystem $S$. Here, to demonstrate the detail of proof process more clearly, the possibility is denoted by $P\left(\rho, O^S := \lambda_j\right)$ with $\rho$ being the state before the measurement.

[2] M. Berta, M. Christandl, R. Colbeck, J. M. Renes, and R. Renner, Nat. Phys. **6**, 659 (2010).
[3] X. Zheng, S. Q. Ma, G. F. Zhang, H. Fan, and W. M. Liu, arXiv:1803.08720 (2018).
[4] W. K. Wootters, Phys. Rev. Lett. **80**, 2245 (1998).
[5] M. Hillery, V. Buzek, and A. Berthiaume, Phys. Rev. A **59**, 1829 (1999).
